# Supplementary material for: Classical Autoencoder Distillation of Quantum Adversarial Manipulations
Source: arXiv:2504.09216 source file (2025-04-12)

— QVC100 — QVC200 — Reconstructed

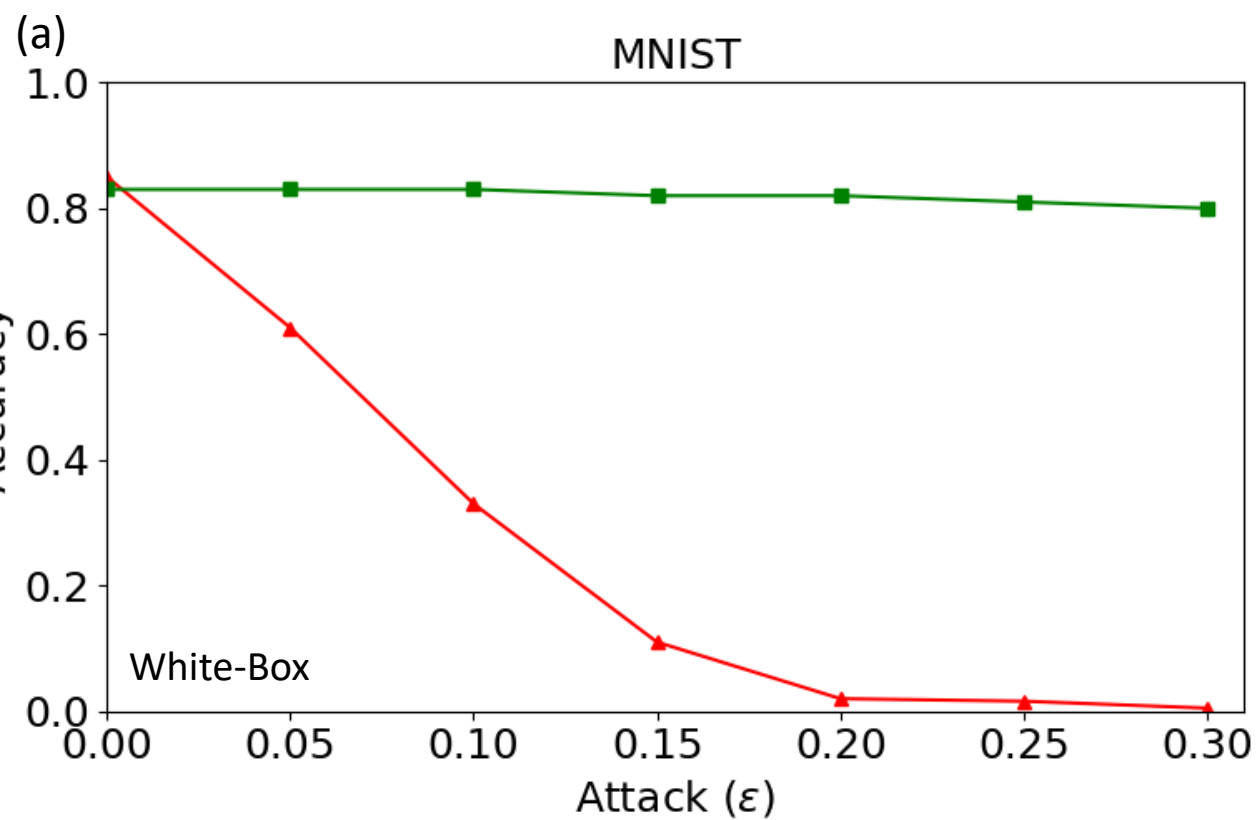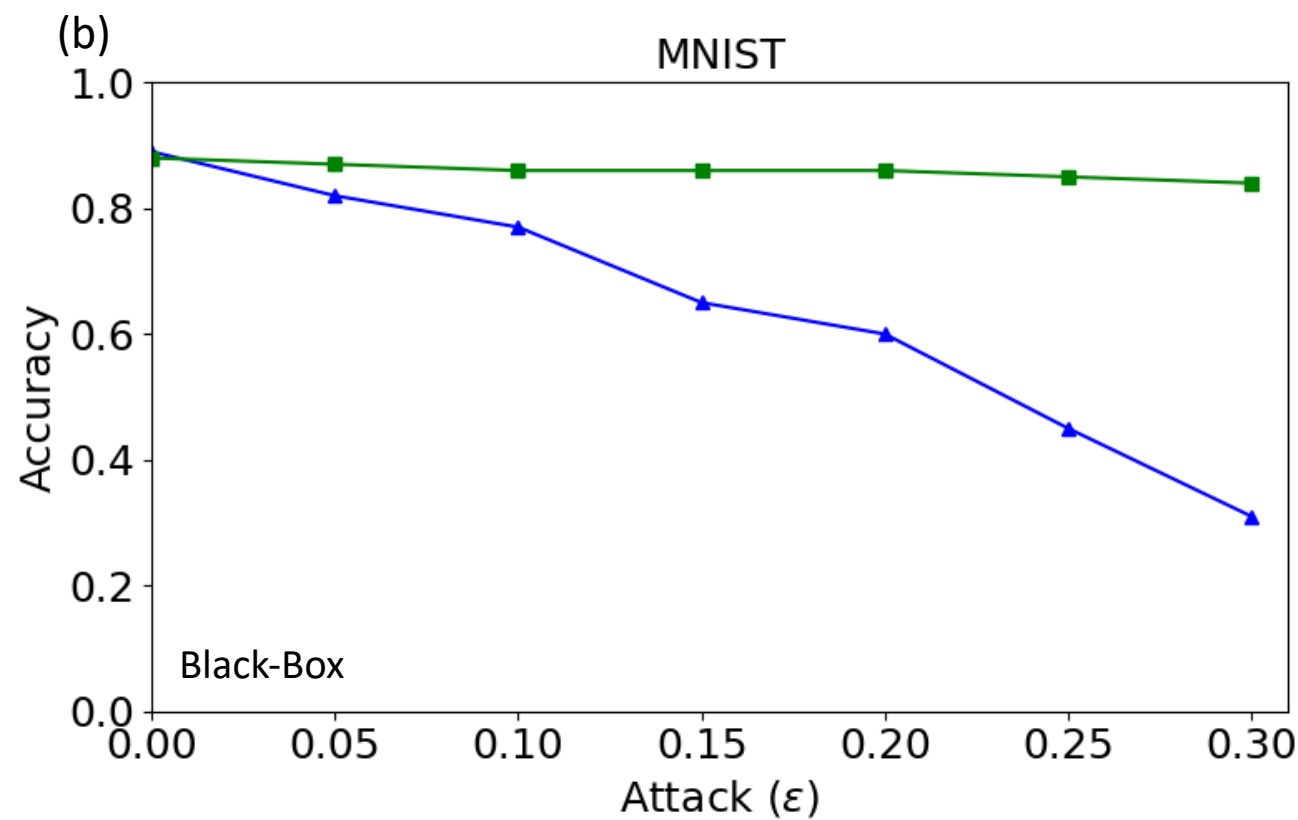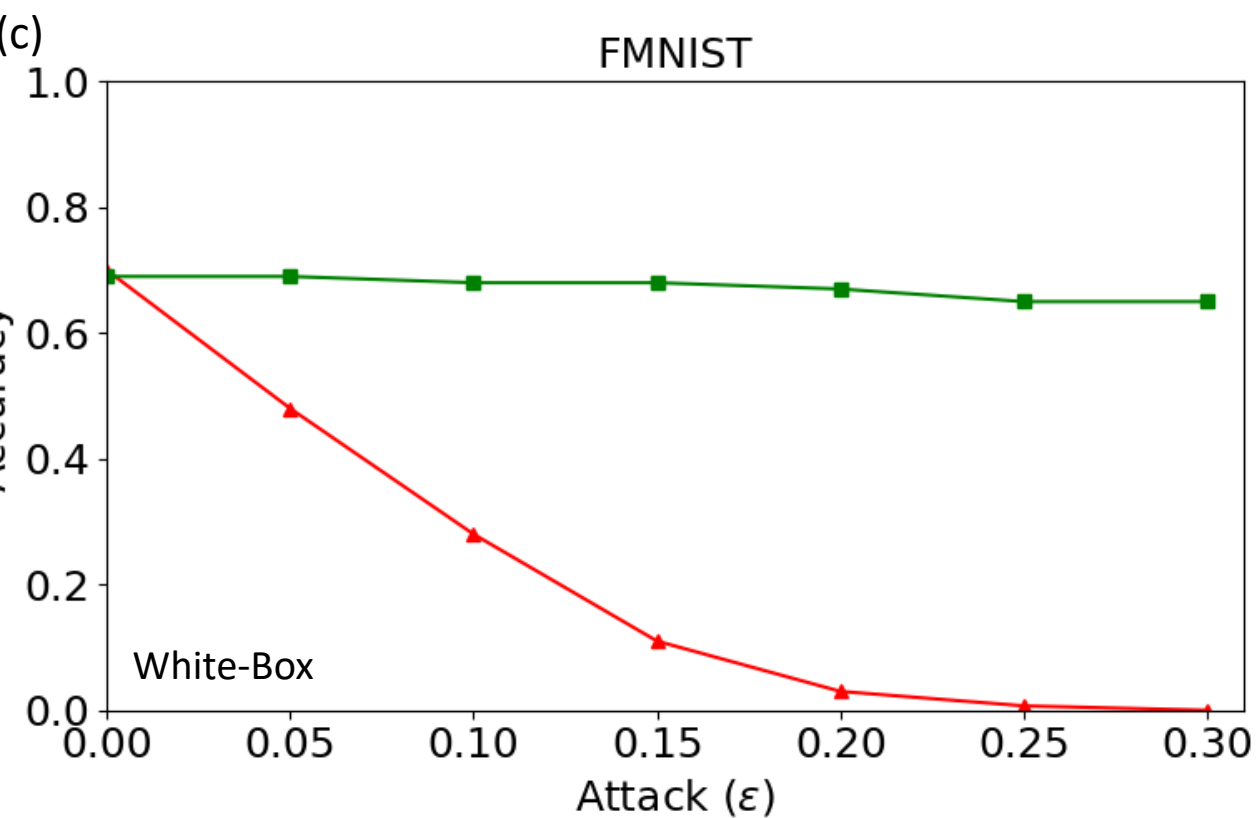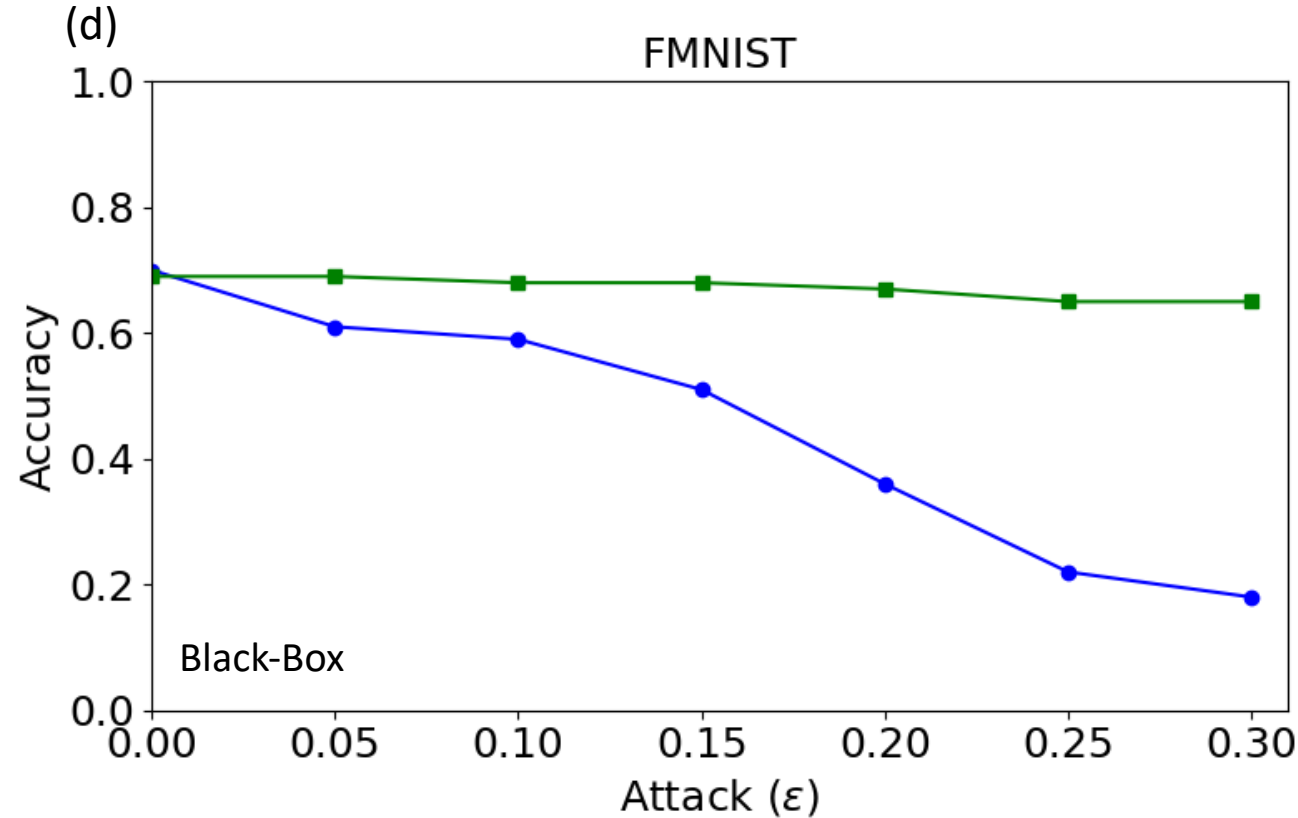

Supplement: Supplementary file 1 [file Graph_17_March.pdf]
